# Supplementary material for: Symmetry and size of membrane protein polyhedral nanoparticles
Source: arXiv:1611.00842 ancillary file (2016-11-02)
Supplement: Supplementary file 1 [file supp.pdf]

# Symmetry and Size of Membrane Protein Polyhedral Nanoparticles
## Supplemental Material

Di Li, Osman Kahraman, and Christoph A. Haselwandter

*Department of Physics & Astronomy and Molecular and Computational Biology Program,*

*Department of Biological Sciences, University of Southern California, Los Angeles, CA 90089, USA*

## STERIC CONSTRAINT ON PROTEIN SEPARATION

To determine the steric constraint on protein separation in our mean-field model of MPPNs we consider neighboring non-overlapping circular membrane patches. As in the main text, we denote the fraction of the surface of a sphere enclosed by $n$ identical non-overlapping circles at closest packing [1] by $p(n)$. We then require that the sum of the areas of the spherical caps enclosed by these circles must be equal to the overall MPPN area multiplied by $p(n)$. Denoting the radius of the non-overlapping circular membrane patches by $\rho'_o$ [2] and the patch boundary angle by $\beta'$, we have $\sin\beta' = \rho'_o/R$. The solid angle enclosed by each patch is given by $2\pi\,(1-\cos\beta')$. Upon equating the area of the $n$ spherical caps to the total MPPN area multiplied by $p(n)$ we find

$$n \times 2\pi R^2 \left[1 - \sqrt{1 - \left(\frac{\rho'_o}{R}\right)^2}\,\right] = 4\pi R^2 p(n) \ . \tag{S1}$$

The steric constraint on protein separation in our mean-field model is then given by $\rho'_o \geqslant \rho_i + \rho_l$, with the membrane patch size $\rho'_o$ defined by Eq. (S1).

## DERIVATION OF MPPN DEFECT ENERGY

### First Approach

The continuum limit of the stretching energy of a hexagonal network of harmonic springs is given by [3]

$$\mathcal{H} = \frac{K}{2} \int d^2x (\nabla \boldsymbol{r})^2 \ , \tag{S2}$$

where $(\nabla \boldsymbol{r})^2 = (\partial \boldsymbol{r}/\partial x_1)^2 + (\partial \boldsymbol{r}/\partial x_2)^2$, in which $x_1$ and $x_2$ are internal coordinates and $\boldsymbol{r} = \boldsymbol{r}(x_1, x_2)$ denotes the external coordinate specifying the location of the surface in the (three-dimensional) embedding space. The continuum force constant $K$ in Eq. (S2) is related to the

discrete force constant $K_0$ of the harmonic springs via $K = \sqrt{3}K_0$ [3]. For a uniform hexagonal lattice of MscS, Eq. (1) of the main text implies [4] the spring constant

$$K_0 = \frac{\pi K_b}{3} \frac{\min(a^4, b^4)}{|a^2 - b^2|\rho_i^2} \,. \tag{S3}$$

To relate Eq. (S2) to the standard stretching energy of a uniform elastic sheet [5] formulated in terms of the areal strain $\Delta A/A$ we consider the position of a point in a flat rectangular patch of an elastic sheet. We denote the width and height of the rectangular patch by $L_1$ and $L_2$, respectively. Now assume that $L_1$ and $L_2$ are extended (or compressed) by $\Delta L_1$ and $\Delta L_2$, respectively. A point in the patch $\boldsymbol{r}_0(x_1, x_2)$ then moves to a new location

$$\boldsymbol{r}(x_1, x_2) = \boldsymbol{r}_0 + \frac{\Delta L_1}{L_1} x_1 \boldsymbol{i} + \frac{\Delta L_2}{L_2} x_2 \boldsymbol{j} \,, \tag{S4}$$

with $\boldsymbol{i}$ and $\boldsymbol{j}$ denoting two orthogonal unit vectors. We therefore have that $(\nabla \boldsymbol{r})^2 = (\partial \boldsymbol{r}/\partial x_1)^2 + (\partial \boldsymbol{r}/\partial x_2)^2 = (\Delta L_1/L_1)^2 + (\Delta L_2/L_2)^2$. For uniform strain we also have that $\Delta L_1/L_1 = \Delta L_2/L_2$, which yields $(\nabla \boldsymbol{r})^2 = 2(\Delta L_1/L_1)^2$. Furthermore, to leading order the area change due to $\Delta L_1$ and $\Delta L_2$ is given by

$$\Delta A = (L_1 + \Delta L_1)(L_2 + \Delta L_2) - L_1 L_2 \approx L_1 \Delta L_2 + L_2 \Delta L_1 \,, \tag{S5}$$

which, again to leading order, yields the squared areal strain

$$\left(\frac{\Delta A}{A}\right)^2 = \left(\frac{\Delta L_1}{L_1} + \frac{\Delta L_2}{L_2}\right)^2 = 4\left(\frac{\Delta L_1}{L_1}\right)^2 = 2(\nabla \boldsymbol{r})^2 \,. \tag{S6}$$

Thus, Eq. (S2) can be expressed in terms of areal strain [5] as

$$\mathcal{H} = \frac{\sqrt{3}K_0}{4} \int d^2x \left(\frac{\Delta A}{A}\right)^2 \,. \tag{S7}$$

For uniform areal strain, $(\Delta A/A)^2$ is a constant and hence [5] can be pulled out of the integral in Eq. (S7). This yields

$$\mathcal{H} = \frac{K_s}{2} A \left(\frac{\Delta A}{A}\right)^2 \,, \tag{S8}$$

where the stretching modulus

$$K_s = \frac{\sqrt{3}K_0}{2} \tag{S9}$$

as in Eq. (2) of the main text. The MPPN defect energy is therefore given by

$$E_d(n, R) = \frac{K_s}{2} A \left(\frac{\Delta A}{A}\right)^2 \,, \tag{S10}$$

where $A = 4\pi R^2$. Similarly as in previous work on viral capsid self-assembly [6], we approximate, at the mean-field level, the areal strain by

$$\frac{\Delta A}{A} = \frac{p_{\max} - p(n)}{p_{\max}}, \tag{S11}$$

where $p(n)$ denotes the fraction of the surface of a sphere enclosed by $n$ identical non-overlapping circles at closest packing [1] and the optimal coverage $p_{\max} = \pi/2\sqrt{3}$ corresponds to hexagonal packing of circular membrane patches. Equation (S3) with Eqs. (S9)–(S11) result in the defect energy $E_d(n, R)$ in Eq. (3) of the main text, with the stretching modulus in Eq. (2) of the main text.

## Second Approach

In our first approach above for deriving the MPPN defect energy in Eq. (3) of the main text we used the result in Ref. [3] that $K = \sqrt{3}K_0$, and then derived the stretching energy in Eq. (S8) from Eq. (S2). To complement this derivation, we obtain here the stretching energy in Eq. (S8) directly from a discrete hexagonal lattice of harmonic springs. In the ground state, we take each triangular element of the lattice, composed of three proteins in the hexagonal spring network, to have side length $r$ with each side corresponding to a harmonic bond. If all three sides of the triangular element are stretched by $\Delta r$, the elastic energy associated with each side is given by $\frac{1}{2}K_0 (\Delta r)^2$. We have three of these bonds per triangle, with each bond shared by two adjacent triangles. The overall energy associated with this area deformation is therefore given by

$$\Delta E_{\text{discrete}} = \frac{1}{2} \times 3 \times \frac{1}{2} K_0 (\Delta r)^2 . \tag{S12}$$

To determine the continuum stretching energy associated with Eq. (S12) we note that the area of an equilateral triangle of side length $r$ is given by $A = \sqrt{3}r^2/4$. To leading order, this implies an area change $\Delta A = \sqrt{3}r\Delta r/2$ due to the stretching deformation $r \to r + \Delta r$. We therefore have that

$$\frac{(\Delta A)^2}{A} = \sqrt{3}(\Delta r)^2 \tag{S13}$$

to leading order. The continuum stretching energy associated with uniform stretching deformations [5] can then be written as

$$\Delta E_{\text{continuum}} = \frac{K_s}{2} \frac{(\Delta A)^2}{A} = \frac{\sqrt{3}K_s}{2} (\Delta r)^2 . \tag{S14}$$

Setting $\Delta E_{\text{continuum}} = \Delta E_{\text{discrete}}$ yields $K_s = \frac{\sqrt{3}}{2} K_0$ as in Eq. (S9), resulting in the stretching modulus in Eq. (2) of the main text and the defect energy $E_d(n, R)$ in Eq. (3) of the main text.

## MSCS TRANSMEMBRANE GEOMETRY

Structural studies suggest [7–9] that the membrane-spanning region of MscS has the shape of a truncated cone. To estimate the cross-sectional radius $\rho_i$ of MscS in the lipid bilayer midplane and the lipid bilayer-MscS contact angle $\alpha$ we rotate the known MscS structure [8] about its symmetry axis normal to the membrane, and fit truncated cones to the MscS transmembrane region (see Fig. S1 for representative snapshots). This yields the estimates $\rho_i \approx 3.2$ nm and $\alpha \approx 0.46$–$0.54$ rad, respectively. We similarly estimate that the length of the MscS cytoplasmic region $\approx 10$ nm.

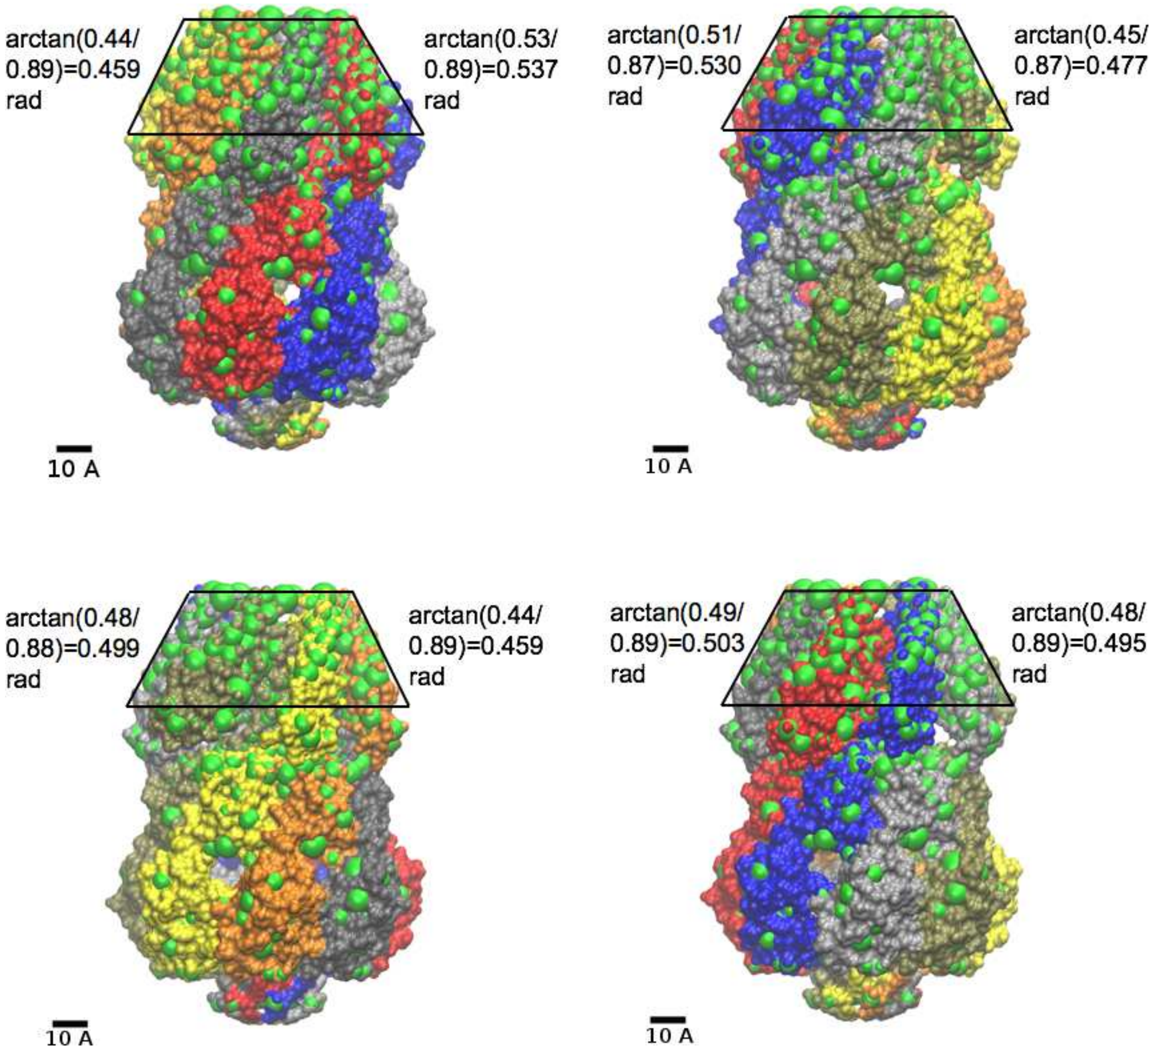


FIG. S1: Molecular structure of MscS in the closed state [8] with Protein Data Bank ID 2OAU represented using Visual Molecular Dynamics [10]. The green beads indicate hydrophobic residues [11] at pH 7. The truncated cones are chosen so as to enclose the approximate transmembrane region of MscS [8, 9]. The values of $\alpha$ quoted in each panel are calculated from the respective truncated cones.

## STRETCHING MODULUS AND MEAN-FIELD MPPN ENERGY

Figure S2(a) shows the stretching modulus $K_s$ in Eq. (2) of the main text as a function of $n$. As $n$ becomes large the MPPN "background curvature" is reduced, which leads to smaller $b$ and hence smaller $K_s$—indeed, in the planar limit, lipid bilayer curvature-mediated interactions are expected to be repulsive [4, 13, 14]. The maximum in $K_s$ is reached for $n$ such that $a \approx b$. Even though the MPPN defect energy in Eq. (3) of the main text is proportional to the overall MPPN area, which tends to increase with $n$, $K_s$ decreases sufficiently rapidly with $n$ so that the MPPN defect energy tends to decrease with $n$ in the large-$n$ regime considered here (see Fig. 2 of the main text). As in Fig. 2 of the main text, Fig. S2(b) shows the minimized total MPPN energy $E_{\text{min}}$ for MPPNs formed from MscS [12] with the contributions $E_b$ and $E_d$ due to bending deformations and packing defects, but over the full $n$-range considered here. The local maximum of $E_{\text{min}}$ at $n = 16$ occurs as a result of the maximum of $K_s$ at $n = 16$ for $\alpha \approx 0.5$ [Fig. S2(a; inset)]. Finally we note that for the MPPNs in Fig. 2 of the main text and Fig. S2(b) we always have that, consistent with the Helfrich-Canham-Evans model [15–17], $|\nabla h| < 1$, where $h(r)$ is the (rotationally-symmetric) height field describing the membrane deformation profile around each protein and $r$ is the radial coordinate [4].

Based on Ref. [4], the divergence in $K_s$ in Eq. (2) of the main text at $a = b$ can be understood as follows. As in Ref. [4], we calculate $K_s$ by differentiating $E_b$ in Eq. (1) of the main text twice with respect to $\rho_o$, and then evaluating this second derivative of $E_b$ at the minimum of $E_b$. For

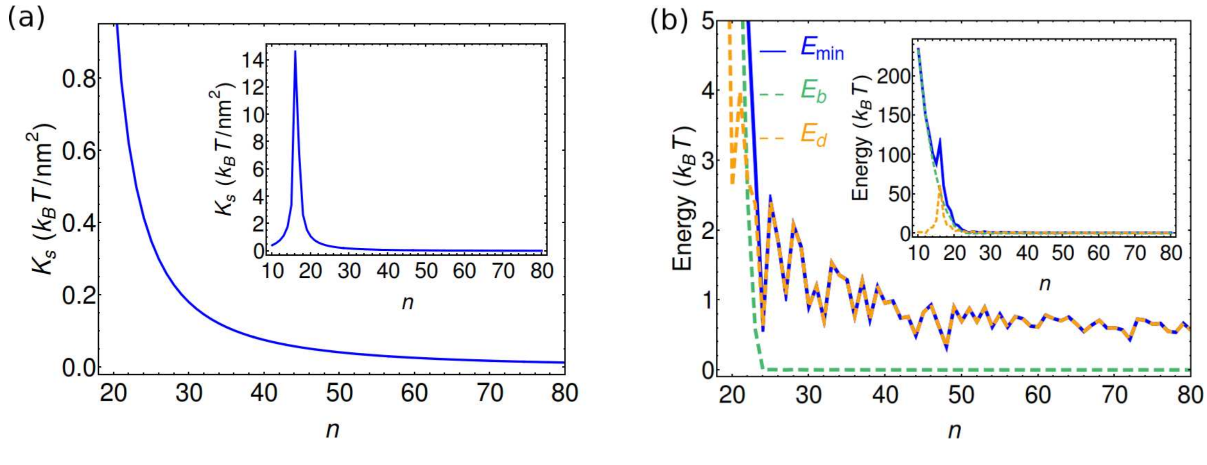


FIG. S2: (a) MPPN stretching modulus $K_s$ and (b) minimized total MPPN energy $E_{\text{min}}$ for MPPNs formed from MscS [12] with the contributions $E_b$ and $E_d$ due to bending deformations and packing defects versus $n$ at $\alpha = 0.5$. The insets in panels (a) and (b) allow for the full $n$-range $10 \le n \le 80$ considered here, while for the main panels we use the same $n$-range as in the main panel of Fig. 2 of the main text.

any $a \neq b$, $E_b$ diverges at $\rho_o = \rho_i$ (this state is unphysical because it corresponds to a vanishing width of the lipid bilayer annulus around each protein; please see the discussion below for further details). As $a \to b$, the minimum in $E_b$ is obtained with $\rho_o \to \rho_i^+$. As $a \to b$, $K_s$ is therefore evaluated at $\rho_o$ which come infinitesimally close to a $\rho_o$ yielding a diverging $E_b$, resulting in a diverging $K_s$. However, as discussed below, this divergence does not affect the central results and predictions of our model. Below, we provide a more detailed discussion of the physical significance and mathematical properties of $E_b$ and $K_s$ as $a \to b$.

We first note that, in each circular membrane patch, the protein-induced lipid bilayer curvature (bending) deformations $h(r)$, where $r$ is the radial coordinate, are given by [4]

$$h(r) = \frac{(r^2 - \rho_i^2)(b\rho_o - a\rho_i) + 2\rho_o\rho_i(a\rho_o - b\rho_i)\ln(r/\rho_i)}{2\left(\rho_o^2 - \rho_i^2\right)}\,, \tag{S15}$$

which, upon substitution into the Helfrich-Canham-Evans bending energy,

$$E_b[h] = \frac{K_b}{2}\int dxdy(\nabla^2 h)^2, \tag{S16}$$

yields, for $n$ membrane patches, the MPPN bending energy in Eq. (1) of the main text:

$$E_b(n,R) = \frac{2n\pi K_b\left(b\rho_o - a\rho_i\right)^2}{\rho_o^2 - \rho_i^2}\,. \tag{S17}$$

For all physically relevant scenarios we must have $\rho_i < \rho_o$. To calculate $K_s$ in Eq. (2) of the main text, we minimize Eq. (S17), at each $n$, with respect to the membrane patch radius $\rho_o$ [18]. We thus find that Eq. (S17) exhibits two extrema:

$$\rho_o^{(1)} = \frac{a}{b}\rho_i\,, \quad \rho_o^{(2)} = \frac{b}{a}\rho_i\,. \tag{S18}$$

The solution $\rho_o^{(1)}$ yields $E_b = 0$, while the solution $\rho_o^{(2)}$ yields a finite $E_b$. Depending on the relative values of $a$ and $b$, we can then distinguish between three cases:

- For $|a| > |b|$ (i.e., $\alpha > \beta$ [19]), the solution $\rho_o^{(1)}$ satisfies $\rho_o^{(1)} > \rho_i$ and is therefore physically relevant, allowing states of minimum bending energy with $E_b = 0$. From Eq. (S15) we see that these states correspond to purely logarithmic radial deformation profiles, resulting in catenoidal lipid bilayer deformations in each membrane patch.

- For $|a| < |b|$ (i.e., $\alpha < \beta$), we have that $\rho_o^{(1)} < \rho_i$ while $\rho_o^{(2)} > \rho_i$. The solution $\rho_o^{(1)}$ is therefore physically irrelevant, the solution $\rho_o^{(2)}$ gives the states of minimum bending energy, and we necessarily have $E_b > 0$. From Eq. (S15) we see that these states correspond to purely quadratic radial deformation profiles, yielding membrane patch deformations that are no longer catenoidal.

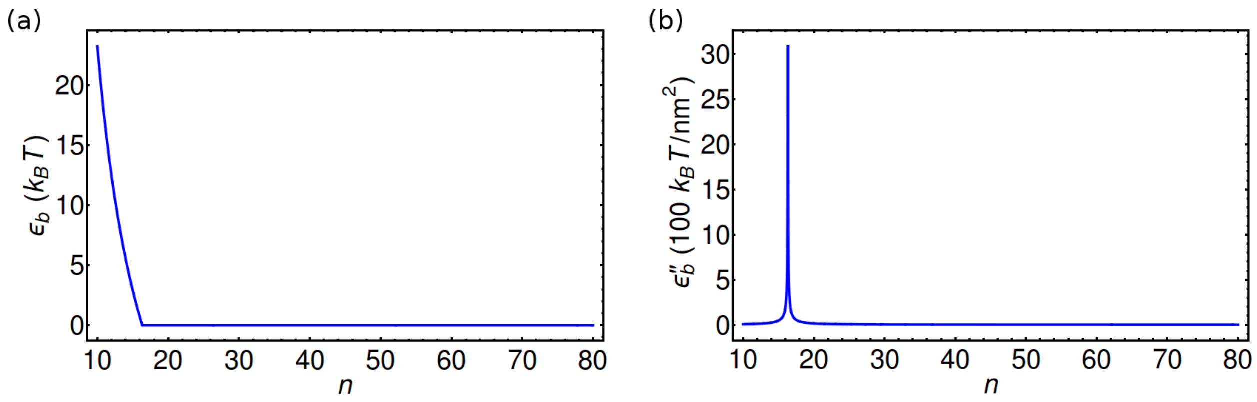


FIG. S3: (a) Numerical values of the minima of the bending energy per membrane patch, $\epsilon_b = E_b(n, R)/n$, obtained by minimizing Eq. (S17) with respect to $\rho_o$ at each $n$, and (b) corresponding second derivatives with respect to $\rho_o$, $\epsilon_b''$, evaluated for each $n$ at the $\rho_o$ minimizing $\epsilon_b$. We used the same parameter values as in Fig. 2 of the main text.

- For $a = b$ (i.e., $\alpha = \beta$), one can still have $E_b = 0$ as the minimum bending energy, but only for the (unphysical) case of a vanishing width of the lipid bilayer annulus, $\rho_i = \rho_o$.

Figure S3 shows the numerical values of the minima of the bending energy per membrane patch, $\epsilon_b = E_b(n, R)/n$, as a function of $n$ (or $b = -\tan\{\arccos[(n-2)/n]\}$, which increases monotonically with $n$ for the range $10 \leq n \leq 80$ we focus on here), together with the corresponding values of its second derivative with respect to $\rho_o$, $\epsilon_b''$, which is proportional to $K_s$ in Eq. (2) of the main text. We find that the divergence in $\epsilon_b''$ and, hence, $K_s$ occurs at $n \approx 16$, at the transition between $\rho_o^{(1)}$ and $\rho_o^{(2)}$ as the physically relevant states of minimum bending energy. Note from Eq. (S17) that, for any $a \neq b$, $E_b$ diverges at $\rho_o = \rho_i$. Since at the transition between the $\rho_o^{(1)}$-branch and the $\rho_o^{(2)}$-branch of the minima of Eq. (S17) we have $\rho_o \to \rho_i^+$, $\rho_o$-states with a finite $E_b$ come infinitesimally close to a $\rho_o$-state with $E_b \to \infty$, yielding a diverging second derivative of $E_b$ with respect to $\rho_o$.

A few remarks are in order here. First we note that, to obtain a "true" divergence of $K_s$, one needs $a = b$. Since $n$ is an integer and, hence, $\beta$ and $b$ are both discretized, $K_s \to \infty$ would require a fine-tuning of $\alpha$. In practice, one therefore only has $a \approx b$, which results in a large, but finite, $K_s$ when transitioning between the $\rho_o^{(1)}$-branch and the $\rho_o^{(2)}$-branch of the minima of Eq. (S17) (see Fig. S3). Furthermore, even if $a$ is fine-tuned to allow $a = b$, this unphysical state is effectively ruled out in our model because it would require an infinite energy. Finally, when calculating the total MPPN energy in Fig. 2 of the main text, we account for steric constraints on lipid and protein size by only allowing for membrane patch sizes $\geqslant \rho_i + \rho_l$, where $\rho_l$ is the lipid radius. This means

that, in the small-$n$ regime $n < n_0$ where one can have $a \approx b$, with $n_0 \approx 20$ for MPPNs formed from MscS [12, 20] with $\alpha \approx 0.5$, the contribution to the total MPPN energy due to bending deformations is large compared to the thermal energy scale $k_B T$ [see Fig. 2 of the main text and Fig. S2(b)]. Thus, the MPPN bending energy already effectively rules out states with $n < n_0$. The divergence in $K_s$ in Eq. (2) of the main text for $a = b$ does therefore not affect the central results and predictions of our model.

The protein-induced lipid bilayer curvature deformations considered here are thought [21–23] to induce non-pairwise-additive bilayer-mediated interactions between proteins. The many-body character of curvature-mediated interactions can potentially have a variety of interesting consequences [23–26], such as stabilization of certain cluster geometries. The mean-field approach we employ here retains, in analogy to planar crystalline lattices [22], some features of the many-body character of curvature-mediated interactions, but does not allow isolation of the possible role of many-body interactions in setting the MPPN symmetry and size. Our mean-field model is motivated by the experimental phenomenology of MPPNs [12], which shows that MPPNs have a spherical shape, and that proteins have an approximately uniform distribution on MPPNs. It was found previously [4] that the mean-field model of MPPN bending energy employed here, which assumes a spherical shape of MPPNs and an approximately uniform distribution of proteins on MPPNs, yields good agreement with computer simulations of budding through interacting conical membrane inclusions or adsorbed, curvature-inducing particles [27, 28]. However, many-body effects not captured by our mean-field approach may, for instance, have interesting consequences for MPPN symmetry and size in situations where the composition of MPPNs is modified to produce departures from approximately uniform protein distributions.

## SIMULATED ANNEALING MONTE CARLO SIMULATIONS

Our mean-field model of MPPNs focuses on long-range (bilayer-mediated) interactions between proteins, and the interaction between the conical protein shape and the spherical geometry of MPPNs. In our minimal molecular model of MPPN organization we consider the complementary scenario of short-range interactions between lipids and proteins, for which we consider a generic (Lennard-Jones) model capturing steric and hydrophobic effects. For our simulated annealing Monte Carlo simulations of our minimal molecular model of MPPN organization we chose protein and lipid parameter values consistent with experiments on MPPNs formed from MscS and diC14:0 lipids [12, 20]. As described in the main text, we represent the lipid bilayer and membrane proteins

by disks lying on the surface of a sphere and assume that lipids interact with other lipids and proteins via Lennard-Jones potentials [29],

$$V_i(r) = \epsilon_i \left[ \left( \frac{\bar{r}_i}{r} \right)^{12} - 2 \left( \frac{\bar{r}_i}{r} \right)^{6} \right] , \tag{S19}$$

with $i = 1, 2$ corresponding to lipid-lipid and lipid-protein interactions, where $r$ is the center-to-center particle distance. For simplicity, we use hardcore steric repulsion for the protein-protein interactions. The $\bar{r}_i$ in Eq. (S19) are the minima of $V_i(r)$ and are determined by the lipid and protein disk sizes. The interaction strengths $\epsilon_i$ in Eq. (S19) can be viewed as the energy penalties for exposing lipids or membrane proteins to an aqueous environment. As discussed below, experiments and previous calculations [30–32] suggest $\epsilon_1 \approx 10\ k_B T$ and $\epsilon_2 \approx 20\ k_B T$ for diC14:0 lipids and MscS in Eq. (S19). To check for robustness of our simulation results we repeated our simulated annealing Monte Carlo simulations for $\epsilon_2/\epsilon_1 = 1$–$10$, and also allowed for unfavorable long-range interactions [13, 14] between MscS, which we calculated analytically for general protein separations using the formalism developed in Refs. [33, 34]. We find that our results regarding the minimum-energy symmetry of MPPNs in Fig. 3 of the main text are not sensitive to the particular value of $\epsilon_2/\epsilon_1$ and protein-protein interactions used.

In our simulated annealing Monte Carlo simulations we took the MPPN sphere radius in our minimal molecular model of MPPN organization to correspond to the hydrophobic-hydrophilic interface in the outer membrane leaflet of MPPNs. The values of the model parameters entering our simulations can then be estimated as follows. We first note that MPPNs formed from diC14:0 lipids and MscS have a lipid:protein ratio $\approx 70$ [12], which yields a total number of lipids $\approx 1700$ for MPPNs with $n = 24$. Experiments suggest [35] that, for lipid bilayer vesicles formed from diC14:0 lipids [12], $\approx 72.5\%$ of the lipids forming the vesicle are located in the outer lipid bilayer leaflet. Assuming that the ratio of lipids in the outer and inner lipid bilayer leaflets in MPPNs [12] is the same as for lipid bilayer vesicles [35], we estimate that the lipid number in the outer MPPN bilayer leaflets $\approx 1200$.

The results in Fig. 3 of the main text correspond to the minimum-energy configuration of MPPNs obtained from our minimal molecular model of MPPN organization for 24 MscS and 1200 lipids in the outer membrane leaflet. We checked for systematic bias by repeating the simulated annealing Monte Carlo simulations in Fig. 3 of the main text with different random seeds. We also repeated our simulations for a range of initial temperatures in the simulated annealing procedure, between five and twenty-five times the room temperature, with Fig. 3 of the main text corresponding to an initial temperature of approximately ten times the room temperature. We used a protein

disk radius $\approx 4.0$ nm corresponding to [8] the outer membrane leaflet of MPPNs and a lipid disk radius $\rho_l \approx 0.45$ nm for diC14:0 lipids [36]. As initial conditions for our simulated annealing Monte Carlo simulations we used non-overlapping but otherwise random configurations of protein disks and random configurations of lipid disks located on the surface of a sphere. We repeated our simulations for sphere radii between 11 nm and 13 nm with step size 0.1 nm. The minimum-energy MPPN configuration in Fig. 3 of the main text was obtained with a sphere radius 12.3 nm which, within the limits of the various approximations made here, is consistent with the corresponding MPPN size obtained from our mean-field model in Figs. 2, 4, and 5 of the main text and observed [12] in experiments on MPPNs formed from MscS and diC14:0 lipids.

To provide simple estimates of the approximate values of $\epsilon_1$ and $\epsilon_2$ in our minimal molecular model of MPPN organization we note that membrane proteins and lipids both have substantial hydrophobic domains, which makes it energetically unfavorable for membrane proteins and lipids to be dissolved in water. We denote by $E_{\text{lipid}}$ the energy required to create the new water-hydrocarbon interface when lipids are dissolved in water. The value of $E_{\text{lipid}}$ can be estimated [30] based on the water-hydrocarbon surface tension $\gamma$ together with the effective area of the contact interface. For simplicity, we approximate [30] the hydrophobic regions of lipids as cylinders of radius $R_{\text{c}}$ and length $n_{\text{cc}} l_{\text{cc}}$, where $n_{\text{cc}}$ is the number of carbon atoms along the lipid hydrocarbon chain and $l_{\text{cc}} = 0.126$ nm [30] is the average C-C bond length along the chain. Therefore, the area of the lipid hydrophobic region $\approx 2\pi n_{\text{cc}} R_{\text{c}} l_{\text{cc}}$, which yields

$$E_{\text{lipid}} \approx 2\pi n_{\text{cc}} R_{\text{c}} l_{\text{cc}} \gamma \,. \tag{S20}$$

For the double-chained diC14:0 lipids used in experiments on MPPNs [12] there are $n_{\text{cc}} = 14$ carbon atoms per hydrocarbon chain, with an effective cross-sectional radius $R_{\text{c}} = 0.3$ nm [30]. Using a water-hydrocarbon surface tension $\gamma \approx 0.02$ J/m$^2$ [30, 37], we thus find $E_{\text{lipid}} \approx 30\ k_B T$ for the two leaflets of a diC14:0 lipid bilayer. Assuming an approximately hexagonal packing of lipids in the lipid bilayer, each lipid has six nearest-neighbor lipids, which yields an effective interaction strength per lipid-lipid bond of $\epsilon_1 \approx \frac{1}{3} E_{\text{lipid}} \approx 10\ k_B T$. To estimate the strength of lipid-protein interactions we assume [31, 32] that the transfer energy of protein residues between polar and hydrophobic media can be estimated based on the water-hydrocarbon surface tension $\gamma$. For proteins such as MscS which are much larger than lipids, one protein can be regarded as substituting for two nearest-neighbor lipids in the approximately hexagonal packing of lipids in the lipid bilayer. This yields an effective interaction strength per lipid-protein bond of $\epsilon_2 \approx \frac{2}{3} E_{\text{lipid}} \approx 20\ k_B T$.

## POLYHEDRAL SYMMETRY OF MPPNS IN MINIMAL MOLECULAR MODEL OF MPPN ORGANIZATION

We define [12] the minimization function used to quantify the quality of the polyhedral fit in Fig. 3 of the main text as the sum over the squared distances between the simulated positions of protein centers in MPPNs and the closest fitted polyhedron vertices. This corresponds to a many-to-one or one-to-many mapping for polyhedra which have fewer or more than 24 vertices, respectively. We used simulated annealing Monte Carlo simulations to minimize the fit error with respect to the following variables: the position of the polyhedron center, the polyhedron size, and the Euler angles. The best fits among the Platonic, Archimedean, Catalan, and Johnson solids obtained via this minimization procedure are summarized in Table I. We find that the snub cube (dextro) provides overall the best fit to the simulated minimum-energy MPPN configuration in Fig. 3 of the main text. We note that in our minimal molecular model of MPPN organization the preference of the minimum-energy configuration for one chiral polyhedral symmetry, such as the snub cube (dextro), rather than its mirror-symmetric configuration, such as the snub cube (levo), only results from the particular (random) initial conditions used. Indeed, repeating the simulations of our minimal molecular model of MPPN organization in Fig. 3 of the main text using the mirror symmetric initial protein configuration we find the snub cube (levo), rather than the snub cube (dextro), as the best fit.

The optimal sphere coverage $p(n)$ [1], plotted in Fig. 2(inset) of the main text, suggests a simple intuitive explanation for our result in Fig. 3 of the main text and Table I that, for $n = 24$, the snub cube yields the minimum-energy MPPN configuration in our minimal molecular model of MPPN organization. From an intuitive perspective it is to be expected that the minimum-energy configuration of lipids and proteins in our minimal molecular model corresponds to a configuration in which proteins are surrounded by lipids so as to maximize favorable lipid-protein interactions, with dense packing of lipids in the intervening space between proteins. One therefore expects that the minimum-energy MPPN configuration in our minimal molecular model of MPPN organization corresponds to an arrangement in which proteins are at the centers of (non-overlapping) circles of maximal radius. This is the protein arrangement implied by $p(n)$ in Fig. 2(inset) of the main text [1] yielding, for $n = 24$, a snub cube symmetry of protein centers as also found in our simulated annealing Monte Carlo simulations of our minimal molecular model of MPPN organization.

| Polyhedron type | Polyhedron | Fit error $\left(\text{Å}^2\right)$ |
|---|---|---|
| A | Snub cuboctahedron (dextro) | 420.2 |
| A | Truncated cuboctahedron | 3724.6 |
| C | Pentagonal hexecontahedron (levo) | 5848.8 |
| C | Pentagonal hexecontahedron (dextro) | 6414.5 |
| J | Gyroelongated square bicupola M2 | 7743.8 |
| A | Rhombicuboctahedron | 7749.3 |
| J | Metabigyrate rhombicosidodecahedron | 8254.4 |
| J | Trigyrate rhombicosidodecahedron | 8841.9 |
| J | Gyroelongated square bicupola M1 | 8877.0 |
| C | Disdyakistriacontahedron | 8947.2 |
| A | Snub icosidodecahedron (levo) | 9107.8 |
| J | Parabigyrate rhombicosidodecahedron | 9181.1 |
| C | Pentagonal icositetrahedron (dextro) | 9289.2 |
| J | Gyrate rhombicosidodecahedron | 9309.3 |
| C | Trapezoidal hexecontahedron | 9425.9 |
| A | Snub cuboctahedron (levo) | 9459.6 |
| J | Elongated square gyrobicupola | 9867.1 |
| A | Rhombicosidodecahedron | 12085.8 |
| C | Pentagonal icositetrahedron (levo) | 12361.2 |
| J | Bigyrate diminished rhombicosidodecahedron | 12455.7 |

TABLE I: Top twenty polyhedral fits to the minimum-energy MPPN configuration in Fig. 3 of the main text predicted by our minimal molecular model of MPPN organization. We define the fit error as the sum over the squared distances between the simulated positions of protein centers and the closest fitted polyhedron vertices. In our fitting procedure we allow for the 132 polyhedral symmetries [38] corresponding to the 5 Platonic solids (P), the 13 Archimedean solids (A) with two chiral pairs, the 13 Catalan solids (C) with two chiral pairs, and the 92 Johnson solids (J) with five chiral pairs.

## MPPN SELF-ASSEMBLY PHASE DIAGRAMS FOR INCREASED LIPID BILAYER BENDING RIGIDITIES AND MODEL EXTENSIONS

It has been suggested [39–41] that the lipid bilayer bending rigidity may be increased in the vicinity of membrane proteins. More generally, the value of the lipid bilayer bending rigidity $K_b \approx 14\ k_BT$ reported for the diC14:0 lipids [42] used for MPPNs [12] lies at the lower end of the range of values of $K_b$ typically measured in experiments on general lipids [9, 42]. We therefore repeated our calculation of the MPPN self-assembly phase diagram in Figs. 4 and 5 of the main text for increased values of $K_b$ (see Figs. S4 and S5). We confirmed that for the dominant MPPNs in Figs. 4 and 5 of the main text and Figs. S4 and S5 we always have that, consistent with the Helfrich-Canham-Evans model [15–17], $|\nabla h| < 1$, where $h(r)$ is the (rotationally-symmetric) height field describing the membrane deformation profile around each protein and $r$ is the radial coordinate [4].

Figures S4(a,b) and S5(a,b) demonstrate that, as the bending rigidity $K_b$ is being increased, the snub cube becomes more and more dominant within the parameter range relevant for MPPNs

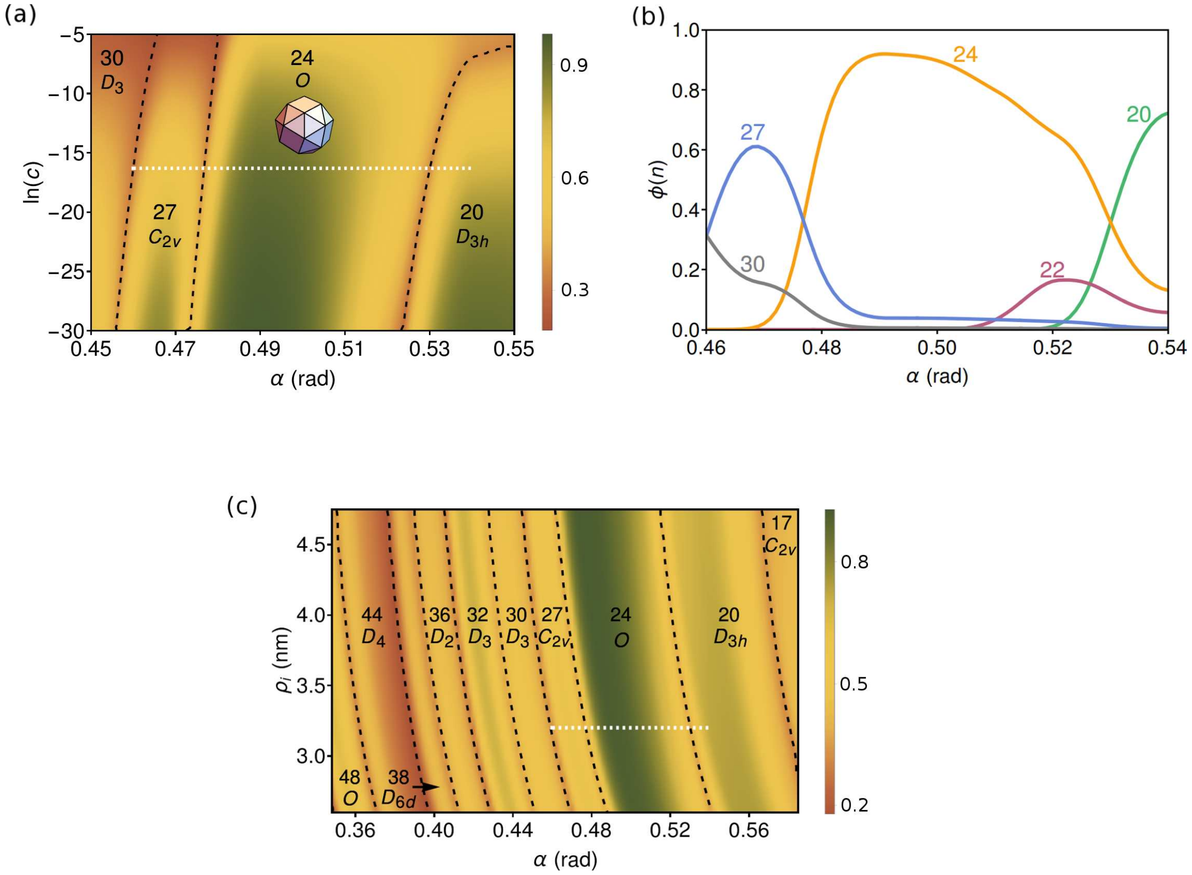


FIG. S4: Same plots as in (a,b) Fig. 4 and (c) Fig. 5 of the main text, but using $K_b = 28\ k_BT$ instead of $K_b = 14\ k_BT$.

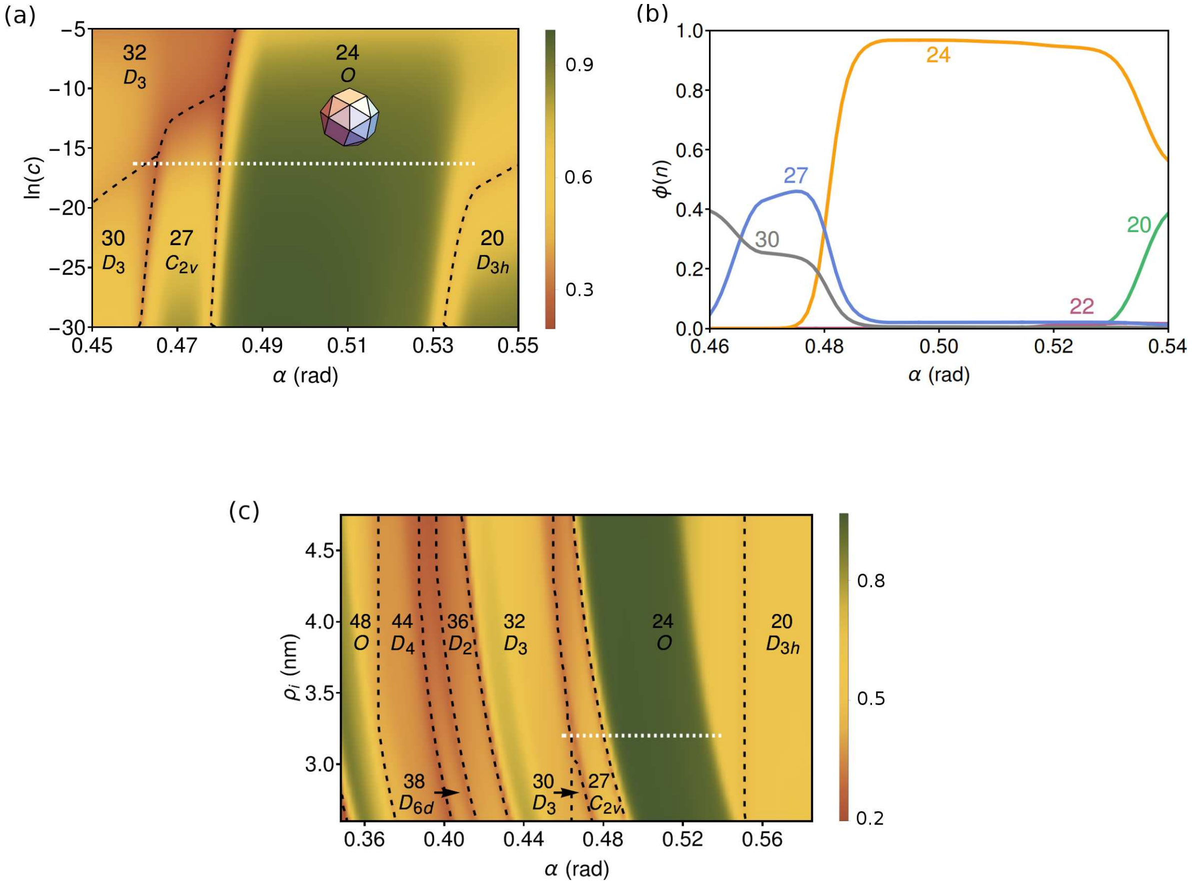


FIG. S5: Same plots as in (a,b) Fig. 4 and (c) Fig. 5 of the main text, but using $K_b = 56\ k_BT$ instead of $K_b = 14\ k_BT$.

formed from MscS [12, 20]. More generally, Figs. S4(c) and S5(c) indicate that a larger $K_b$ yields a stronger preference for close packing of proteins. This can be understood by noting that, for small $K_b$, the energy differences between different $n$-states of MPPNs are small in the large-$n$ regime dominated by the MPPN defect energy (see, e.g., Fig. 2 of the main text), which allows strong thermal effects. In contrast, large $K_b$ tend to produce large magnitudes of the MPPN defect energy in the large-$n$ regime, increasingly biasing the MPPN self-assembly phase diagram towards states with (locally) optimal packing of proteins. Finally we note that the MPPNs with $n = 24$ obtained along the white dashed lines in Figs. S4 and S5, which correspond to experiments on MPPNs formed from MscS [12, 20], have the same approximate size as the corresponding MPPNs with $n = 24$ in Figs. 4 and 5 of the main text.

In addition to changes in the value of the lipid bilayer bending rigidity, we have also checked the robustness of the predicted MPPN self-assembly phase diagram with respect to changes in membrane tension. To this end, we generalized our analytic model of MPPN self-assembly to allow

for a finite membrane tension as captured by the Helfrich-Canham-Evans energy [15–17],

$$G_h[h] = \frac{1}{2}\int dxdy \left[K_b(\nabla^2 h)^2 + \tau(\nabla h)^2\right] \,, \tag{S21}$$

where $\tau$ is the membrane tension. An upper value for the membrane tension in MPPNs formed from (closed) MscS [12, 20] is given by the MscS gating tension $\tau \approx 1.3\ k_BT/\mathrm{nm}^2$ [43]. For this value of the membrane tension we find, using the values of $\alpha$, $\rho_i$, and $c$ relevant for experiments on MPPNs formed from MscS [12, 20] and discussed in the main text, that the observed snub cube symmetry of MPPNs [12] becomes even more dominant than in the MPPN self-assembly phase diagram in Figs. 4 and 5 of the main text, and that our model predicts the same approximate size of the dominant MPPNs with $n = 24$ as in the case of zero membrane tension. Our results pertaining to the dominant symmetry and size of MPPNs are therefore robust with respect to changes in membrane tension.

We finally note that, as far as the use of MPPNs for structural studies is concerned, it is desirable to produce MPPNs that have a uniform polyhedral symmetry and size. As shown in Figs. 4 and 5 of the main text as well as Figs. S4 and S5, small $\alpha$ tend to yield large $n$. In the large-$n$ regime, different $n$-states of MPPNs do not show substantial differences in the optimal sphere coverage $p(n)$ [Fig. 2(inset) of the main text]. This generally leads to non-uniform MPPN symmetries, i.e., broad distributions of $n$-states, which is expected to decrease the resolution of MPPN-based approaches for the structural analysis of membrane proteins. Our model suggests possible strategies for overcoming this practical limitation. In particular, our model suggests that MPPNs with smaller $n$ are produced if the effective $\alpha$ is increased. This could be achieved, for instance, through addition of suitable toxins [9] that localize to the lipid bilayer-protein interface and amplify protein-induced lipid bilayer bending deformations. Furthermore, in addition to bending deformations, membrane proteins may also induce thickness deformations in the surrounding lipid bilayer. Through appropriate tuning of the competition between protein-induced lipid bilayer bending and thickness deformations (via, for instance, changes in the lipid tail length) it may be possible to stabilize MPPNs with reduced $n$. We will address the generalization of our model of MPPN self-assembly to include thickness deformations, as well as a finite membrane tension, in a separate publication.

---

[1] B. W. Clare and D. L. Kepert, J. Math. Chem. **6**, 325 (1991).

[2] The variable $\rho_o$ ($> \rho_o'$) in the main text corresponds to overlapping membrane patches [4, 44] and, as such, is less convenient for defining a suitable steric constraint on protein separation.

[3] Y. Kantor, M. Kardar, and D. R. Nelson, Phys. Rev. A **35**, 3056 (1987).

[4] T. Auth and G. Gompper, Phys. Rev. E **80**, 031901 (2009).

[5] R. Phillips, J. Kondev, J. Theriot, and H. Garcia, *Physical Biology of the Cell* (Garland Science, London and New York, 2012).

[6] R. F. Bruinsma, W. M. Gelbart, D. Reguera, J. Rudnick, and R. Zandi, Phys. Rev. Lett. **90**, 248101 (2003).

[7] R. B. Bass, P. Strop, M. Barclay, and D. C. Rees, Science **298**, 1582 (2002).

[8] S. Steinbacher, R. Bass, P. Strop, and D. C. Rees, Curr. Top. Membr. **58**, 1 (2007).

[9] R. Phillips, T. Ursell, P. Wiggins, and P. Sens, Nature **459**, 379 (2009).

[10] W. Humphrey, A. Dalke, and K. Schulten, J. Mol. Graphics **14**, 33 (1996).

[11] O. D. Monera, T. J. Sereda, N. E. Zhou, C. M. Kay, and R. S. Hodges, J. Pept. Sci. **1**, 319 (1995).

[12] T. Basta, H.-J. Wu, M. K. Morphew, J. Lee, N. Ghosh, J. Lai, J. M. Heumann, K. Wang, Y. C. Lee, D. C. Rees, et al., Proc. Natl. Acad. Sci. U.S.A. **111**, 670 (2014).

[13] M. Goulian, R. Bruinsma, and P. Pincus, Europhys. Lett. **22**, 145 (1993).

[14] T. R. Weikl, M. M. Kozlov, and W. Helfrich, Phys. Rev. E **57**, 6988 (1998).

[15] W. Helfrich, Z. Naturforsch. **28C**, 693 (1973).

[16] P. Canham, J. Theor. Biol. **26**, 61 (1970).

[17] E. Evans, Biophys. J. **14**, 923 (1974).

[18] This is equivalent to minimizing $E_b$ with respect to $R$ since $\rho_o = R \sin \beta$, with $\beta$ fixed for each $n$.

[19] We have that $a = -\tan \alpha$ and $b = -\tan \beta$, with $\alpha$ set by the particular protein under consideration and $\beta = \arccos[(n-2)/n]$.

[20] H.-J. Wu, T. Basta, M. Morphew, D. C. Rees, M. H. B. Stowell, and Y. C. Lee, Micro Nano Lett. **8**, 672 (2013).

[21] K. S. Kim, J. Neu, and G. Oster, Biophys. J. **75**, 2274 (1998).

[22] J.-B. Fournier, Eur. Phys. J. B. **11**, 261 (1999).

[23] S. Weitz and N. Destainville, Soft Matter **9**, 7804 (2013).

[24] P. Dommersnes and J.-B. Fournier, Eur. Phys. J. B **12**, 9 (1999).

[25] K. S. Kim, J. C. Neu, and G. F. Oster, Europhys. Lett. **48**, 99 (1999).

[26] K. S. Kim, T. Chou, and J. Rudnick, Phys. Rev. E **78**, 011401 (2008).

[27] E. Atılgan and S. X. Sun, J. Chem. Phys. **121**, 10392 (2004).

[28] B. J. Reynwar, G. Illya, V. A. Harmandaris, M. M. Müller, K. Kremer, and M. Deserno, Nature **447**, 461 (2007).

[29] R. Zandi, D. Reguera, R. F. Bruinsma, W. M. Gelbart, and J. Rudnick, Proc. Natl. Acad. Sci. U.S.A. **101**, 15556 (2004).

[30] D. H. Boal, *Mechanics of the Cell* (Cambridge University Press, Cambridge, 2012), 2nd ed.

[31] N. Ben-Tal, A. Ben-Shaul, A. Nicholls, and B. Honig, Biophys. J. **70**, 1803 (1996).

[32] S. Choe, K. A. Hecht, and M. Grabe, J. Gen. Physiol. **131**, 563 (2008).

[33] C. A. Haselwandter and R. Phillips, Europhys. Lett. **101**, 68002 (2013).

[34] C. A. Haselwandter and N. S. Wingreen, PLoS Comput. Biol. **10**, e1003932 (2014).

[35] B. De Kruijff, P. Cullis, and G. Radda, BBA-Biomembranes **406**, 6 (1975).

[36] K. V. Damodaran and K. M. Merz, Langmuir **9**, 1179 (1993).

[37] V. A. Parsegian, T. Faraday Soc. **62**, 848 (1966).

[38] G. Hart, The Encyclopedia of Polyhedra, www.georgehart.com/virtual-polyhedra/vp.html, 2000.

[39] M. B. Partenskii and P. C. Jordan, J. Chem. Phys. **117**, 10768 (2002).

[40] T. Kim, K. I. Lee, P. Morris, R. W. Pastor, O. S. Andersen, and W. Im, Biophys. J. **102**, 1551 (2012).

[41] K. I. Lee, R. W. Pastor, O. S. Andersen, and W. Im, Chem. Phys. Lipids **169**, 19 (2013).

[42] W. Rawicz, K. Olbrich, T. McIntosh, D. Needham, and E. Evans, Biophys. J. **79**, 328 (2000).

[43] S. Sukharev, Biophys. J. **83**, 290 (2002).

[44] M. M. Müller and M. Deserno, Prog. Theor. Phys. Supp. **184**, 351 (2010).
